# Supplementary material for: A Proof of $\mathfrak{L}^2$-Boundedness for Magnetic Pseudodifferential Super Operators via Matrix Representations With Respect to Parseval Frames
Source: arXiv:2405.19964 source file (2024-05-30)
Supplement: Supplementary file 1 [file appendix.tex]

%!TEX root = ./humble boundedness super PsiDOs.tex
%
\begin{appendix}
	\section{Basic definitions and properties of Parseval frames} % (fold)
	\label{appendix:parseval_frames}
	%
	
	% section basic_definitions_and_properties_of_parseval_frames (end)
\end{appendix}
